# Supplementary material for: Tunable Cooperativity in Coupled Spin--Cavity Systems
Source: arXiv:2102.11713 ancillary file (2021-02-23)
Supplement: Supplementary file 1 [file CSO-Resonator-Latex_SI.pdf]

# Supplemental Material: Tunable Cooperativity in Coupled Spin–Cavity Systems

Lukas Liensberger,<sup>1,2,\*</sup> Franz X. Haslbeck,<sup>3</sup> Andreas Bauer,<sup>3</sup> Helmuth Berger,<sup>4</sup>  
Rudolf Gross,<sup>1,2,5</sup> Hans Huebl,<sup>1,2,5</sup> Christian Pfeiderer,<sup>3,5</sup> and Mathias Weiler<sup>1,2,6,†</sup>

<sup>1</sup>*Walther-Meißner-Institut, Bayerische Akademie der Wissenschaften, 85748 Garching, Germany*

<sup>2</sup>*Physik-Department, Technische Universität München, 85748 Garching, Germany*

<sup>3</sup>*Lehrstuhl für Topologie korrelierter Systeme, Physik-Department,*

*Technische Universität München, 85748 Garching, Germany*

<sup>4</sup>*Institut de Physique de la Matière Complexe, École Polytechnique Fédérale de Lausanne, 1015 Lausanne, Switzerland*

<sup>5</sup>*Munich Center for Quantum Science and Technology (MCQST), 80799 Munich, Germany*

<sup>6</sup>*Fachbereich Physik and Landesforschungszentrum OPTIMAS,  
Technische Universität Kaiserslautern, 67663 Kaiserslautern, Germany*

(Dated: February 23, 2021)

# $\text{Cu}_2\text{OSeO}_3$ CRYSTAL, LOOP-GAP RESONATOR AND BACKGROUND SUBTRACTION

Image of  $\text{Cu}_2\text{OSeO}_3$  Crystal and Loop-Gap Resonator

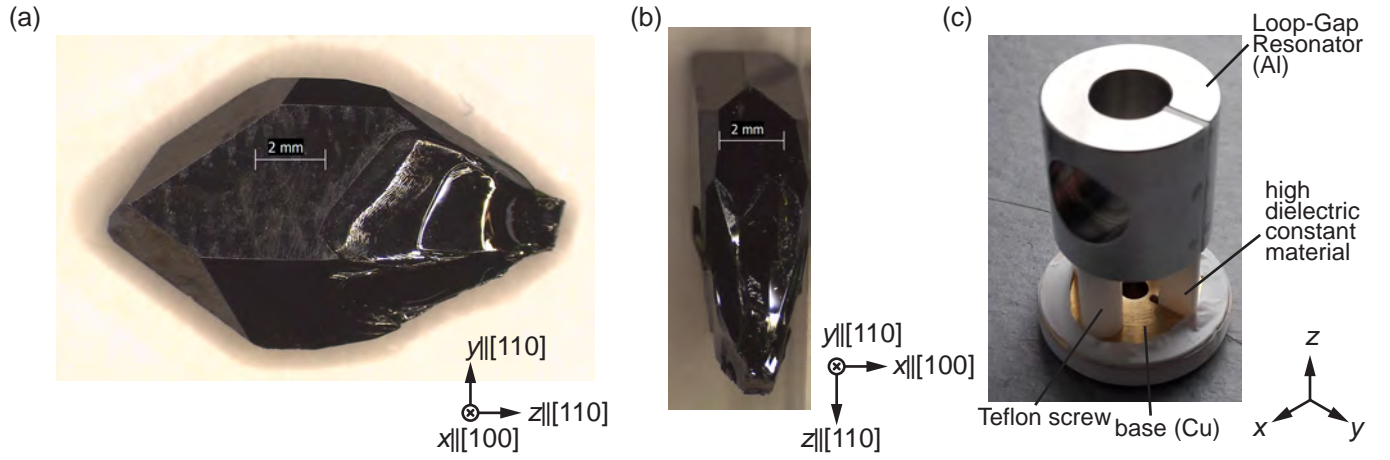

FIG. S1. (a),(b) Images of the investigated  $\text{Cu}_2\text{OSeO}_3$  single-crystal in (a) top view and (b) side view. The maximum dimensions of the main axis of the crystal are  $l_x = 3.38$  mm,  $l_y = 7.71$  mm and  $l_z = 12.89$  mm. (c) Image of the loop-gap resonator with the high dielectric constant material (Rogers Corporation RO3010) in the gap. The aluminum (Al) made resonator is mounted with Teflon screws to the base where it is brought in vicinity of the self-designed feedline using a rotatable radiation shield (not shown).

# Finite-element Simulations of Loop-Gap Resonator

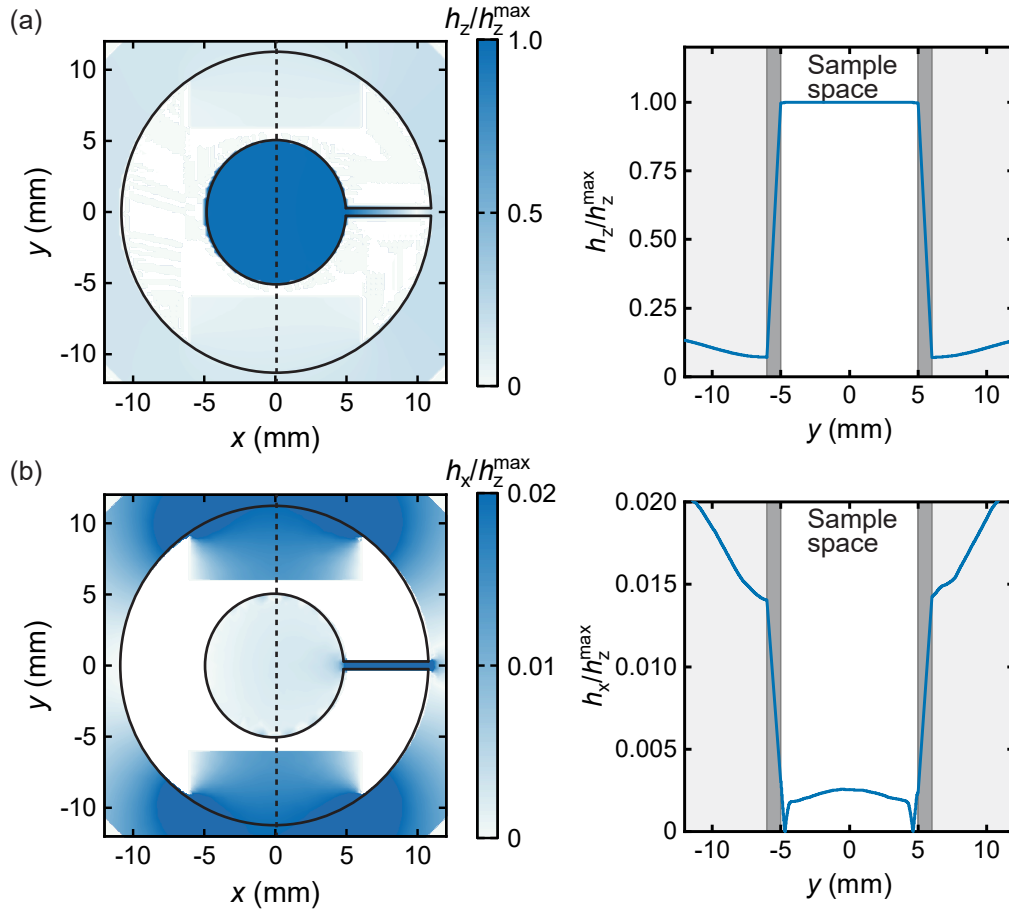

FIG. S2. Finite-element simulation of the magnetic field inside the loop-gap resonator performed with CST microwave studio. Magnetic field strength of (a) the out-of-plane component  $h_z$  and (b) the in-plane component  $h_x$  normalized to the maximum field  $h_z^{\max} = \max(h_z)$  in the center of the microwave cavity where the sample is placed. The solid black lines indicate the contour of the loop-gap resonator. The dark gray shaded area indicates the aluminum and in light gray the space outside the resonator (air). In the right column a cut through the center of the cavity (indicated by the dashed black line in the left figures) is shown, demonstrating the homogeneity the magnetic field inside the microwave cavity. The magnetic field  $h_z$  at the sample location varies by less than 1% over the whole sample space.

## Background Subtraction of Cavity Magnetic Resonance Data

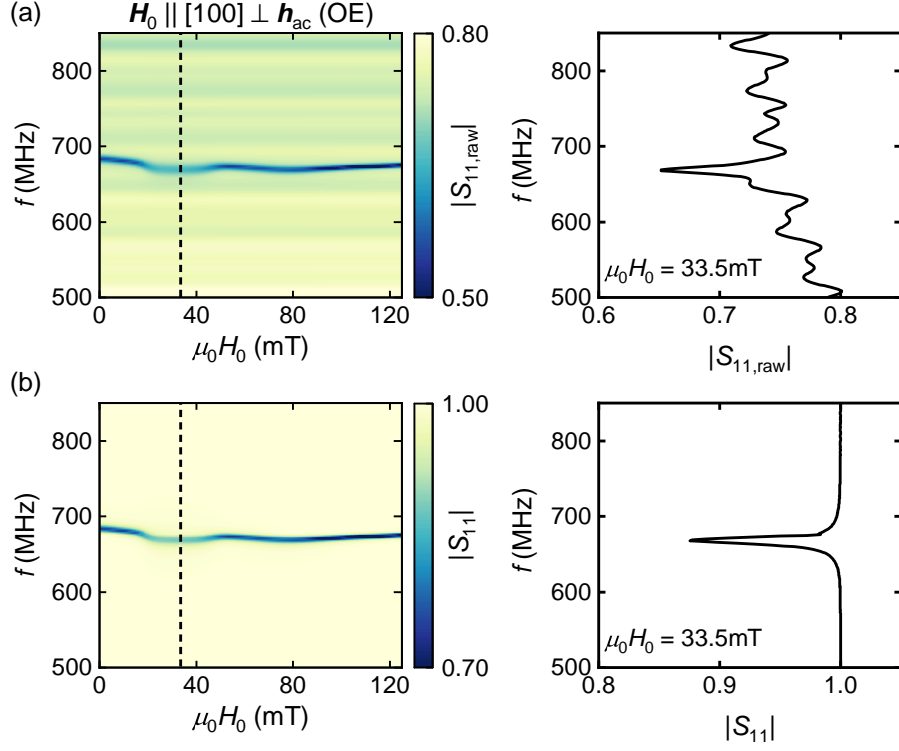

FIG. S3. (a) Measured complex reflection parameter  $S_{11,\text{raw}}$  of the loaded system (cavity and  $\text{Cu}_2\text{OSeO}_3$  crystal) with a vector network analyzer (Rohde&Schwarz ZVA8) without any background correction to eliminate the standing wave pattern of the microwave equipment due to small impedance mismatch in the setup. The dashed black line shows the magnetic field ( $\mu_0 H_0 = 33.5 \text{ mT}$ ) where the frequency trace is extracted from. To eliminate the field-independent microwave background a piece-wise defined function  $S_{\text{bg}}$  is defined, where we take frequency-traces at magnetic fields where no resonance of the cavity is observable [1]. The measured  $S_{11,\text{raw}}$  is then divided by the newly defined function  $S_{11} = S_{11,\text{raw}}/S_{\text{bg}}$ . The result is shown in panel (b) with the corresponding frequency-trace at  $\mu_0 H_0 = 33.5 \text{ mT}$ . This data is the same as shown in the main text in Fig. 3(b) but with an extended frequency range.

# BROADBAND FERROMAGNETIC RESONANCE SPECTROSCOPY

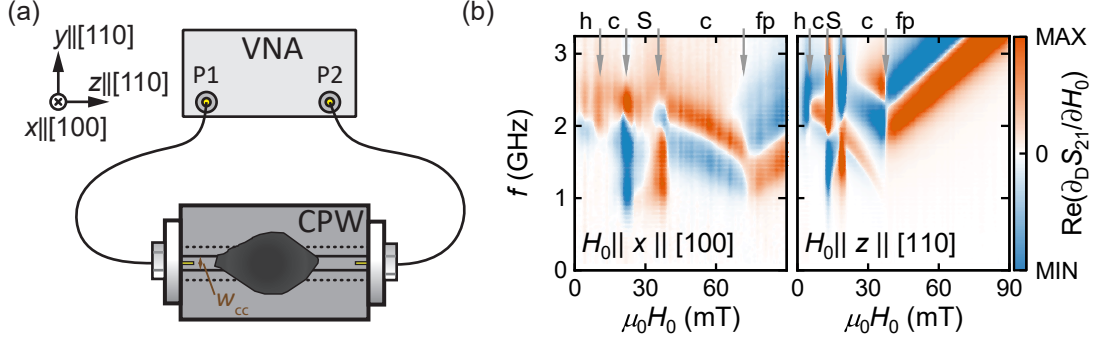

FIG. S4. (a) Schematic of the broadband magnetic resonance (BMR) spectroscopy setup where the  $\text{Cu}_2\text{OSeO}_3$  crystal is placed on the coplanar waveguide (CPW). (b) Exemplary microwave background-corrected BMR data of  $S_{21}$  for  $\mathbf{H}_0 \parallel x \parallel [100]$  and  $\mathbf{H}_0 \parallel z \parallel [110]$  at  $T = 56.5 \text{ K}$ . Here, the background-corrected field-derivative of the complex transmission parameter  $\partial_D S_{21} / \partial H_0$  is shown, which is calculated using Eq. (S1). The phase boundaries are indicated with gray arrows. Note that the phase transition from the conical (c) to skyrmion lattice phase (S) is not sharp due to the inhomogeneous demagnetization fields stemming from the irregular shape of the single-crystal.

For the determination of the resonance frequency  $f_{\text{mag}}$  and the magnon loss rate  $\kappa_{\text{mag}}$ , we perform broadband magnetic resonance (BMR) spectroscopy using a coplanar waveguide (CPW) and a vector network analyzer (VNA). A schematic depiction of the experimental setup is shown in Fig. S4(a). The  $\text{Cu}_2\text{OSeO}_3$  crystal is placed on the CPW and a static magnetic field  $\mathbf{H}_0$  is applied. The vector network analyzer (VNA) generates a microwave at port 1 (P1) with frequency  $f$  and power  $P = 0 \text{ dBm}$ . The microwave is coupled into the center conductor (width  $w_{\text{cc}} = 340 \mu\text{m}$ ) of the CPW by using endlaunch connectors where the microwave generates an oscillating driving field by Ampere's law to excite the magnetization dynamics. The VNA measures the complex transmission parameter  $S_{21}$  at port 2 (P2) for various magnetic fields  $H_0$  and frequencies  $f$  [2, 3].

Exemplary data with the external magnetic field  $\mathbf{H}_0$  applied along  $\mathbf{H}_0 \parallel x \parallel [100]$  and  $\mathbf{H}_0 \parallel z \parallel [110]$  at  $T = 56.5 \text{ K}$  is shown in Fig. S4(b). To eliminate the frequency-dependent microwave background, the magnetic field derivative [4]

$$\partial_D S_{21} / \partial H_0 = \frac{S_{21}(H_0 + \Delta H) - S_{21}(H_0 - \Delta H)}{S_{21}(H_0) \Delta H}, \quad (\text{S1})$$

is calculated, where  $\Delta H$  is the fixed magnetic field step, which in our case is  $\mu_0 \Delta H = 0.3 \text{ mT}$ .

The data is fitted in the same procedure as proposed in Refs. [4, 5] and the extracted resonance frequencies  $f_{\text{mag}}$  and half-width-at-half-maximum linewidth corresponding to the magnon loss rate  $\kappa_{\text{mag}}$  are shown in Figs. S5 and S6 respectively. The extracted magnetic field-dependence of  $f_{\text{mag}}$  is fitted in the field-polarized (fp) and in the conical phase (c) using the analytical formulas proposed in Refs. [6, 7]. In the skyrmion lattice phase (S) and in the helical phase (h) there are no analytical formulas to describe  $f_{\text{mag}}$  vs.  $H_0$ , so the magnetic field-dependence of  $f_{\text{mag}}$  is fitted to a linear function. In the phase transition region (yellow shaded area), we linearly interpolate between the last extracted value of  $f_{\text{mag}}$  in the skyrmion lattice phase and in the conical phase. For the magnon decay rates  $\kappa_{\text{mag}}$ , the data is fitted using  $\kappa_{\text{mag}} / 2\pi = \alpha \cdot f_{\text{mag}} + \Delta f$  with a damping parameter  $\alpha$  and an inhomogeneous linewidth  $\Delta f$ . The results for  $f_{\text{mag}}$  and  $\kappa_{\text{mag}}$  are shown as solid black lines in Fig. S5 and S6 respectively. These values of the fitted functions are used in the fits in the main text for  $f_{\text{mag}}$  and  $\kappa_{\text{mag}}$ .

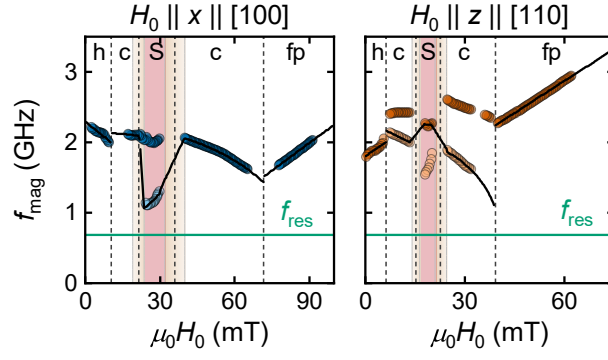

FIG. S5. Experimentally extracted resonance frequencies  $f_{\text{mag}}$  by BMR spectroscopy (c.f. Fig. S4) as a function of the applied magnetic field magnitude  $H_0$  with the external field applied along the  $x$ -direction (left panel) and  $z$ -direction (right panel). The error bars are smaller than the symbol size. The resonance frequencies  $f_{\text{mag}}$  are extracted by fitting frequency traces of the background-corrected transmission parameter  $\partial_D S_{21}/\partial H_0$  at fixed magnetic field  $H_0$  to Eq. (5) in Ref. [4]. Note that the skyrmion lattice phase (S) is indicated by the red shaded area and there is no sharp transition from and to the conical phase (c) observable, indicated by the yellowish shading. The solid black lines are fits to the magnetic field dependent  $f_{\text{mag}}$  as described in the text. This function is used in the input-output formalism for  $f_{\text{mag}}$ .

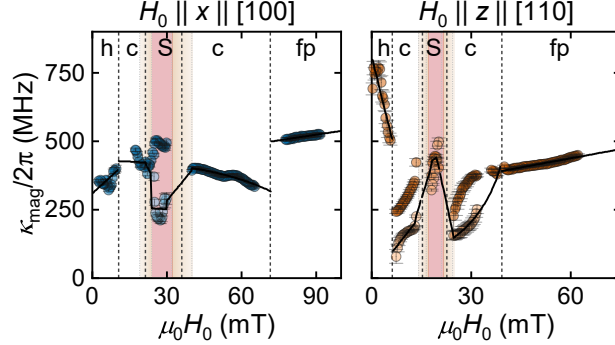

FIG. S6. Experimentally extracted half-width-at-half-maximum linewidths corresponding to the magnon decay rate  $\kappa_{\text{mag}}$  by BMR spectroscopy (c.f. Fig. S4) as a function of the applied magnetic field magnitude  $H_0$  with the external field applied along the  $x$ -direction (left panel) and  $z$ -direction (right panel). The magnon loss rate  $\kappa_{\text{mag}}$  are extracted by fitting frequency traces of the background-corrected transmission parameter  $\partial_D S_{21}/\partial H_0$  at fixed magnetic field  $H_0$  to Eq. (5) in Ref. [4]. Note that the skyrmion lattice phase (S) is indicated by the red shaded area and there is no sharp transition from and to the conical phase (c) observable, indicated by the yellowish shading. The solid black lines are fits to the magnetic field dependent  $\kappa_{\text{mag}}$  as described in the text. This function is used in the input-output formalism for  $\kappa_{\text{mag}}$ .

# ADDITIONAL REFLECTION MEASUREMENTS OF CAVITY-MAGNON SYSTEM

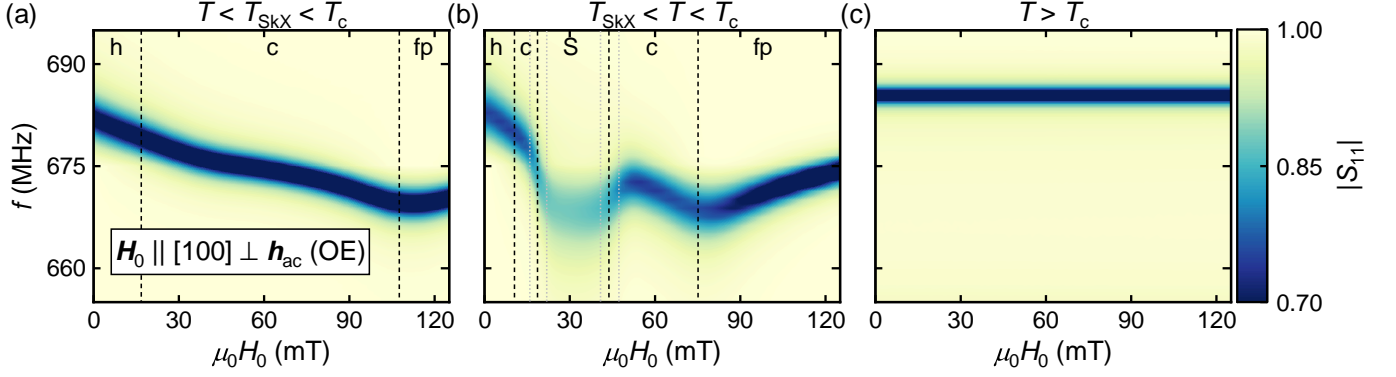

FIG. S7. Additional measurements of the background-corrected reflection parameter  $|S_{11}|$  at different temperatures for the external magnetic field is applied along the OE case ( $\mathbf{H}_0 \parallel [100] \perp \mathbf{h}_{ac}$  (OE)). (a) The temperature is chosen too low for the skyrmion lattice phase to be able to form ( $T < T_{\text{SkX}} < T_c$ ). (b) The temperature is close to the transition temperature ( $T_c \approx 58$  K) where magnon-photon coupling in the skyrmion lattice phase (**S**) is observed. Due to the irregular shape of the crystal and therefore inhomogeneous demagnetization fields, the phase transition from the conical (**c**) to the skyrmion lattice phase (**S**) is not sharp, indicated by the dashed gray lines. Note that this is the same data as in the main text. (c) The temperature is chosen larger than the transition temperature  $T_c$  where the crystal has no magnetic order anymore. In this regime the magnetic field-independent cavity resonance is observed.

\* Lukas.Liensberger@wmi.badw.de

† weiler@physik.uni-kl.de

- [1] L. V. Abdurakhimov, S. Khan, N. A. Panjwani, J. D. Breeze, M. Mochizuki, S. Seki, Y. Tokura, J. J. L. Morton, and H. Kurebayashi, Magnon-photon coupling in the noncollinear magnetic insulator Cu<sub>2</sub>OSeO<sub>3</sub>, Phys. Rev. B **99**, 140401 (2019).
- [2] S. S. Kalarickal, P. Krivosik, M. Wu, C. E. Patton, M. L. Schneider, P. Kabos, T. J. Silva, and J. P. Nibarger, Ferromagnetic resonance linewidth in metallic thin films: Comparison of measurement methods, J. Appl. Phys. **99**, 093909 (2006).
- [3] I. Neudecker, G. Woltersdorf, B. Heinrich, T. Okuno, G. Gubbiotti, and C. Back, Comparison of frequency, field, and time domain ferromagnetic resonance methods, J. Magn. Magn. Mater. **307**, 148 (2006).
- [4] H. Maier-Flaig, S. T. B. Goennenwein, R. Ohshima, M. Shiraishi, R. Gross, H. Huebl, and M. Weiler, Note: Derivative divide, a method for the analysis of broadband ferromagnetic resonance in the frequency domain, Rev. Sci. Instrum. **89**, 076101 (2018).
- [5] S. Klingler, V. Amin, S. Geprägs, K. Ganzhorn, H. Maier-Flaig, M. Althammer, H. Huebl, R. Gross, R. D. McMichael, M. D. Stiles, S. T. B. Goennenwein, and M. Weiler, Spin-Torque Excitation of Perpendicular Standing Spin Waves in Coupled YIG/Co Heterostructures, Phys. Rev. Lett. **120**, 127201 (2018).
- [6] T. Schwarze, J. Waizner, M. Garst, A. Bauer, I. Stasinopoulos, H. Berger, C. Pfleiderer, and D. Grundler, Universal helimagnon and skyrmion excitations in metallic, semiconducting and insulating chiral magnets, Nat. Mater. **14**, 478 (2015).
- [7] M. Weiler, A. Aqeel, M. Mostovoy, A. Leonov, S. Geprägs, R. Gross, H. Huebl, T. T. M. Palstra, and S. T. B. Goennenwein, Helimagnon Resonances in an Intrinsic Chiral Magnonic Crystal, Phys. Rev. Lett. **119**, 237204 (2017).
